# Supplementary material for: CORE: a Complex Event Recognition Engine
Source: arXiv:2111.04635 source file (2022-05-26)
Supplement: Supplementary file 1 [file app-exp-uniform.tex]

\renewcommand{\T}{\texttt{T}}

\noindent \textbf{Sequence queries with output.} We start by considering sequence queries, which have been used for benchmarking in CER before (see, for example, \cite{SASE,SASEcomplexity,cayuga,WPI,SAPesp}). Specifically, we consider sequence patterns of length $n$ occurring within time window $\T$ of the form:
\begin{verbatim}
	SELECT * FROM RandomStream
	WHERE A1 ; A2 ; ... ; An
	WITHIN T
\end{verbatim}
where \texttt{A1} to \texttt{An} are $n$ events of different types. \texttt{RandomStream} is a stream of $n+6$ possible event types, namely, \texttt{A1} to \texttt{An} plus \texttt{B1} to \texttt{B6}. The input stream is randomly generated, such that  each event type  appears with uniform probability $\frac{1}{n+6}$. We use \texttt{B1} to \texttt{B6} to introduce noise, in the form of irrelevant events. Although systems can easily discard these events as non-relevant to the query, they affect the probability that a complex event occurs in the time window.

\begin{figure*}[t]
	\centering
	\includegraphics[width=17.5cm]{../plots/seq-uniform}
	\vspace{-3mm}
	\caption{The throughput (top-left), update throughput (top-right), enumeration throughput (bottom-left), and memory consumption (bottom-right) of evaluating sequence queries of length 3, 5, 7 and 9 with windows length of 100 events.}
	\label{plot:seq}
\end{figure*}

\begin{figure*}[t]
	\centering
	\includegraphics[width=17.5cm]{../plots/seq-nomatch-uniform}
	\vspace{-3mm}
	\caption{At the left, the throughput of sequence query \texttt{A1;A2;A3} with time windows of 50, 100, 150, and 200 events, respectively, and without outputs. At the right, the throughput of the same sequence query with time window 100 under selection strategies.}
	\label{plot:seq-nomatches}
\end{figure*}

\renewcommand{\oom}{OOM\xspace}

In Figure~\ref{plot:seq}, we display the results of evaluating sequence queries of length $n = 3, 5, 7, 9$ and a fixed time window size $\T = 100$ events. The top-left plot shows the throughput, in logarithmic scale, grouped by system. \systemname's throughput is in the order of $10^6$ e/s, while that of Esper and FlinkCEP is  one to three orders of magnitude (\oom) lower. When $n =3$ or $n=5$, SASE's throughput  is higher than CORE.  However, as $n$ grows, SASE's performance degrades exponentially. In contrast, CORE's throughput is stable, and degrades only linearly in $n$. For $n=9$ CORE outperforms SASE by 6x, Esper by 33x, and FlinkCEP by 500x.

The top-right and bottom-left of Figure~\ref{plot:seq} separate the throughput in update throughput (updates per second) and enumeration throughput (outputs per second). On the one hand, the throughput of all systems improves when we remove the enumeration time. Nevertheless, the degrading behavior of SASE is more evident in this plot. The enumeration throughput of CORE is comparable (even slightly higher) to that of  Esper and FlinkCEP, while being lower than that of SASE. Since CORE stores the output compactly in the tECS data structure (see Section~\ref{sec:evaluation}), it needs to ``decompress'' each result before enumeration. Instead, SASE maintains each output explicitly, making the enumeration procedure more direct and faster. Although the output-linear delay approach forces CORE to pay this cost, it pays off regarding the overall throughput.  

The bottom-right of Figure~\ref{plot:seq}  shows the memory consumption for each query and system. The memory used by CORE is high ($\sim$200MB) but stable in $n$. Instead, the memory consumption of  Esper, FlinkCEP\footnote{The memory consumption of FlinkCEP drops for $n=7,9$. This is because in these cases FlinkCEP processes significantly less events compared to other systems, and compared to lower values of $n$.} and SASE grows exponentially in $n$.

\smallskip
\noindent \textbf{Sequence queries without output.} The previous experiment considers sequence queries in the setting where the sought pattern occurs frequently in the randomly generated input stream. Because we adopt the consumption policy that forgets all input events seen so far once a matched complex event is found, this implies that, on average, the different systems need to remember only a limited set of partial answers. In practice, however, we may expect CER systems to look for unusual events, which means that the number of partial answers that need to be remembered may be significantly larger. Our next experiment captures this setting.
We fix the sequence pattern \texttt{A1; A2; A3} (i.e., $n = 3$, the case with the highest throughput for all systems in the previous experiment) and vary the window size from $\T=50$ to $\T=200$. We generate a random input stream with event types \texttt{A1}, \texttt{A2}, \texttt{B1}, $\ldots$, \texttt{B6}, each with uniform probability. The event type \texttt{A3} that fires a complex event is not included. We are therefore at the extreme point where systems look for an unusual complex event that never appears.

In Figure~\ref{plot:seq-nomatches} (left) we show the throughput (log scale) for each window size, grouped by system. We see that CORE outperforms other systems by at least one \oom when $\T=50$ and by three \oom when $\T=200$ (more than 3800 times faster than SASE). This is in stark contrast with the frequent-match setting of the previous experiment, where SASE outperforms CORE.  Note that we are still using relatively small time windows, of at most 200 events; in practice windows may be significantly larger. We also observe that the performance of other systems degrades exponentially in  the time size $T$. Indeed, this is clear for Esper, where the throughput is more than $10^5$ e/s when $\T=50$ but less than $10^4$ e/s when $\T=200$. In contrast, CORE is stable.% , and degrades slowly when the size of the time windows increases. 
%Although the theoretical analysis says that the time window should not affect the algorithm's performance, we can explain this cost by the memory consumption of keeping the active window in the main memory, which requires more resources when $\T$ increases. 

\begin{figure*}[t]
	\centering
	\includegraphics[width=8.5cm]{../plots/oper} \ \ \ \ \
    \includegraphics[width=8.5cm]{../plots/stock}
	\vspace{-2mm}
	\caption{At the left: the throughput of evaluating queries with iteration ($K3$ and $K5$) and disjunction ($D3$ and $D5$) with a time window of $100$ events. At the right: The throughput of evaluating queries $Q_1$ to $Q_7$ over stock market stream.}
	\label{plot:other-operators}
       	\label{plot:stock}
\end{figure*}

\smallskip
\noindent \textbf{Selection strategies.} Many CER systems offer so-called selection strategies~\cite{DBLP:journals/vldb/GiatrakosAADG20,cugola2012, SASE,SASEcomplexity}. % One could disregard previous experiments by arguing that, in practice, users do not look for all possible outputs, and systems aid this search by providing the so-called selection strategies. 
A selection strategy can be seen as a heuristic for evaluating a query, where the system is asked to return only a specific subset of all matched complex event. Since this subset is often easier to recognize, it improves performance.
In the next experiment, we compare all systems in the presence of  selection strategies. Unfortunately, each system has its own algorithm for selection strategy and, thus, it is not possible to guarantee that everyone generates the same outputs. To solve this, we keep the approach of the previous experiment, namely, a sequence query \texttt{A1;A2;A3} and $\T = 100$, where we hide the last event \texttt{A3}. In this setting, there is no output, and we  argue that all systems are hence performing the same task; namely, we test the case where the selection strategy found no result (i.e., an unusual event). Nevertheless, the systems are still free to adopt their performance-improving heuristics, consistent with their selection strategy.

The throughput (log scale) of the four systems with selection strategies is shown in Figure~\ref{plot:seq-nomatches} (right). CORE implements four different selection strategies: ALL (no selection strategy), NEXT, LAST, and MAX (see~\cite{CELJOURNAL} for the semantics of each selection strategy). All are implemented at the automata level, doing a sophisticated determinization procedure to filter outputs, namely, the algorithm is the same (see Section~\ref{sec:evaluation}), but the underlying automaton is different. We used the default selection strategy for the other systems. 

From Figure~\ref{plot:seq-nomatches} we can conclude that the use of a selection strategy improves the performance of Esper, FlinkCEP, and SASE. The last system is the one that has a better improvement, going from $10^3$ e/s (without selection strategy) to  $10^4$ e/s (with selection strategy). Despite this improvement, CORE is two \oom above other systems (i.e., $10^6$ e/s) in all selection strategies. We can conclude then that the advantage of CORE is in the  evaluation algorithm rather than in the use of selection strategies. 

\smallskip
\noindent \textbf{Other operators.} We next consider queries with iteration and disjunction. For testing iteration, we consider the patterns
$$
\text{K3}\ := \ \texttt{A1;A2+;A3} \ \ \ \text{ and  } \ \ \ 
\text{K5} \ := \ \texttt{A1;A2+;A3;A4+;A5}
$$
which are the natural extensions of sequence queries with $n=3$ and $n=5$. Similarly, for disjunction, we use queries:
$$
\begin{array}{l}
	\text{D3} \ := \ \texttt{A1;(A2 OR A2');A3} \ \ \ \ \text{ and } \\
	\text{D5} \ := \ \texttt{A1;(A2 OR A2');A3;(A4 OR A4');A5}.
\end{array}
$$
We set $\T = 100$, and we randomly generate the input stream to contain 
 query's event types plus \texttt{B1} to \texttt{B6} (i.e., noise) with uniform probability. Note that this experiment produces outputs similar to the first experiment (``sequence queries with output'').

Figure~\ref{plot:other-operators} (left) shows the throughput (log-scale) per query,
grouped by system. There is no result on D3 and D5 for SASE, given that it does
not support queries with
disjunction. % From this plot, we can infer two conclusions.
We first observe that CORE outperforms all other systems by 2 or 3 \oom on
queries with iteration and disjunction. Furthermore, CORE's performance is
stable, maintaining a throughput of over one million events per second on all
queries. The throughput of other systems, in contrast, degrades significantly as
we increase the query length. All of this is consistent with the observations of
the previous experiments. 
Second, when we compare Figure~\ref{plot:other-operators} with Figure~\ref{plot:seq} we see that adding iteration or disjunction  affects the throughput of all systems except \systemname, which remains stable around $10^6$ e/s. For example, the throughput of Esper and SASE on the sequence query \texttt{A1;A2;A3} is around $10^6$ e/s, but drops two \oom to  $10^4$ e/s  when adding an iteration (K3).  Note that this analysis does not consider the time windows size, which we know also negatively impacts the throughput of all systems except CORE. 

\smallskip
\noindent \textbf{Stock market data.} We next compare systems on real-world data consisting of stock market events.\footnote{\url{https://davis.wpi.edu/datasets/Stock_Trace_Data/}}
This dataset has already been  used in the past to compare  CER systems ~\cite{PoppeLAR17,PoppeLRM17,DBLP:conf/sigmod/PoppeLR019,PoppeLMRR21}. Similar to Example~\ref{ex:cer-hard}, the stream contains \texttt{BUY} and \texttt{SELL} events  of stocks in a single market day, ordered by timestamp. Each event also has the stock name, volume and price (see Example~\ref{ex:cer-hard}). We test seven queries containing different features and measure the throughput of each system. Given space restrictions, we present the full CEQL definition of each query in the online appendix~\cite{system}, and limit ourselves here to the the following simplified description.
% . Instead, we give here a brief description of each query. For a quick reference, we provide the following table with a simplified description of each query.
%\stijn{Didn't we replicated the events a number of times? Shouldn't this be mentioend?}
\begin{center}
\small
	\begin{tabular}{|l|}
		\hline
		$Q_1$ \ := \ \texttt{SELL} ; \texttt{BUY} ; \texttt{BUY} ; \texttt{SELL} \\ \hline
		$Q_2$ \ := \  $Q_1$ + \texttt{FILTER} \\ \hline
		$Q_3$ \ := \  $Q_1$  + \texttt{PARTITION BY} \\ \hline
		$Q_4$ \ := \  \texttt{SELL} ; \texttt{(BUY OR SELL)} ; \texttt{(BUY OR SELL)} ; \texttt{SELL} \\ \hline
		$Q_5$ \ := \  $Q_4$  + \texttt{FILTER} \\ \hline
		$Q_6$ \ := \  $Q_4$  + \texttt{PARTITION BY} \\ \hline
		$Q_7$ \ := \  \texttt{SELL} ; \texttt{(BUY OR SELL)}+ ; \texttt{SELL} \\
		\hline
	\end{tabular}
\end{center}

% \begin{figure*}[t]
% 	\centering
% 	\includegraphics[width=17.5cm]{../plots/stock}
% 	\vspace{-2mm}
% 	\caption{The throughput of evaluating queries $Q_1$ to $Q_7$ over stock market stream.}
% 	\label{plot:stock}
% \end{figure*} 

% We translate each query into the corresponding query language of the competing systems, preserving the semantics with some exceptions.
As we already mentioned, SASE does not support disjunction, and  we hence omit $Q_4$--$Q_7$ for SASE. Queries $Q_3$ and $Q_6$ use the partition-by clause. Unfortunately, every system gave different outputs when we tried partition-by queries. Therefore, for $Q_3$ and $Q_6$ we cannot guarantee query equivalence for all systems. % Despite this, we maintain both queries for testing partition-by queries, although the outputs are incomparable. 
In all other cases, the results provided by each system are the same.  

In Figure~\ref{plot:stock} (right) we show the throughput (log-scale), grouped per query. The figure confirms our observations of the previous experiments. % From this plot, we can confirm several hypotheses that we claimed previously.
Over real data, CORE's throughput is stable (i.e., $10^6$ e/s) and approximately two \oom faster than other systems, which are not stable. % Again,  CORE's throughput is stable for all queries (i.e., $10^6$ e/s), while that of the other systems vary. Another observation we can confirm over real data is that certain operators 
Also, the presence of certain operators (e.g., filters or disjunction) may decrease  performance, except for CORE. For example, disjunction decreases the performance of Esper (e.g., compare $Q_1$ and $Q_4$). Interestingly, adding filters reduces the performance of some systems like, for example, SASE on $Q_1$ and $Q_2$, or Esper on $Q_4$ and $Q_5$. CORE does not suffer from these problems due to its automaton-based evaluation algorithm. % , given that we compiled the query into an automaton, and we use a single algorithm that guarantees the same performance for every automaton.
Finally, we can see that partition-by aids the performance of systems like Esper and SASE but slightly decreases the throughput of CORE and FlinkCEP (see $Q_3$ and $Q_6$). For CORE, we evaluate the partition-by clause by running several instances of the main algorithm, one for each partition, which diminishes the throughput. Nevertheless,  CORE still outperforms the competition.

%%% Local Variables:
%%% mode: latex
%%% TeX-master: "../main/main"
%%% End:
