# Supplementary material for: CORE: a Complex Event Recognition Engine
Source: arXiv:2111.04635 source file (2022-05-26)
Supplement: Supplementary file 2 [file semantic-differences.tex]

\stijn{To Alejandro: please add some  examples where smantics (ours vs e.g. sase) is different. Suggestion from Cristian: with projection, or with IN}

%%% Local Variables:
%%% mode: latex
%%% TeX-master: "../main/main"
%%% End:
